# Supplementary material for: Test-Time Strategies for More Efficient and Accurate Agentic RAG
Source: arXiv:2603.12396 source file (2026-03-12)
Supplement: Supplementary file 1 [file appendix.tex]

\appendix

\section{Appendix}
\label{sec:appendix}

\subsection{Sample Output From Search-R1}
\begin{tcolorbox}[colback=gray!5!white, breakable, enhanced]
\textbf{Question:} Who was appointed to the board of supervisors first, Jeff Sheehy or Ed Lee?

\textcolor{blue}{<think>} I need to determine if Jeff Sheehy or Ed Lee was appointed to the board of supervisors first. I'll search for it.\textcolor{blue}{</think>}

\textcolor{cyan}{<search>} who was appointed to the board of supervisors first, Jeff Sheehy or Ed Lee \textcolor{cyan}{</search>}

\textcolor{orange}{<information>} Doc 1(Title: "Jeff Sheehy") Jeff Sheehy \textbf{Jeff Sheehy} is a former member of the San Francisco Board of Supervisors representing Supervisorial District 8. He was appointed to the Board in \textbf{January 2017 by then-mayor Ed Lee} ...
Doc 2(Title: "Jeff Sheehy") ...Following Scott Wiener's departure from the San Francisco Board of Supervisors due to his election to the California State Senate in 2016, Sheehy was appointed to fill out the remainder of his term by San Francisco Mayor Ed Lee...
Doc 3(Title: "Ed Lee (politician)") ... At the January 7 meeting, the old board voted 10–1 to elect Lee as mayor, with outgoing Supervisor Chris Daly casting the lone ""no"" vote...
\textcolor{orange}{</information>}

\textcolor{blue}{<think>} I found out that Jeff Sheehy was appointed to the San Francisco Board of Supervisors. Now I need to find out if Ed Lee was appointed before or after Jeff Sheehy. \textcolor{blue}{</think>}

\textcolor{cyan}{<search>} when was Ed Lee appointed to the board of supervisors \textcolor{cyan}{</search>}

\textcolor{orange}{<information>} 
Doc 1(Title: "Ed Lee (politician)") take their place.) The Board of Supervisors nominated four people — former Mayor Art Agnos, Sheriff Michael Hennessey, former Board of Supervisors President Aaron Peskin, and Lee. ... At the January 7 meeting, the old board voted 10–1 to elect Lee as mayor ...
Doc 2(Title: "Ed Lee (politician)") Ed Lee (politician) ... He took office as San Francisco city administrator in 2005 and was appointed on January 11, 2011 by the Board of Supervisors to serve out the remaining term of former Mayor Gavin Newsom ...
Doc 3(Title: "Ed Lee (politician)") if appointed, a statement that helped to gain support for his appointment. ...
\textcolor{orange}{</information>}

\textcolor{blue}{<think>} I found out that Ed Lee was appointed as the Mayor of San Francisco. Now I need to find out if he was appointed to the board of supervisors before Jeff Sheehy. \textcolor{blue}{</think>}

\textcolor{cyan}{<search>} when was Jeff Sheehy appointed to the board of supervisors \textcolor{cyan}{</search>}

\textcolor{orange}{<information>}...\textcolor{orange}{</information>}

\textcolor{blue}{<think>} I found out that Jeff Sheehy was appointed to the San Francisco Board of Supervisors in January 2017. Now I need to find out if Ed Lee was appointed before or after Jeff Sheehy. \textcolor{blue}{</think>}

\textcolor{cyan}{<search>} when was Ed Lee appointed to the board of supervisors \textcolor{cyan}{</search>}

\textcolor{orange}{<information>}...\textcolor{orange}{</information>}

\textcolor{blue}{<think>} I found out that Ed Lee was appointed as the Mayor of San Francisco on January 11, 2011. Now I can compare the appointments of Ed Lee and Jeff Sheehy to the board of supervisors. \textcolor{blue}{</think>}

\textcolor{purple}{<answer>} Ed Lee \textcolor{purple}{</answer>}

\textbf{\textcolor{teal}{Correct Answer:}} Ed Lee
\end{tcolorbox}

\subsection{Sample Output From Search-R1 With GPT-4.1-mini Information Extractor}
\begin{tcolorbox}[colback=gray!5!white, breakable, enhanced]
\textbf{Question:} Who was appointed to the board of supervisors first, Jeff Sheehy or Ed Lee?

\textcolor{blue}{<think>} I need to determine if Jeff Sheehy or Ed Lee was appointed to the board of supervisors first. I'll search for it. \textcolor{blue}{<think>}

\textcolor{teal}{<search>} who was appointed to the board of supervisors first, Jeff Sheehy or Ed Lee \textcolor{teal}{</search>}

\textcolor{orange}{<retrieval>}Doc 1(Title: "Jeff Sheehy") Jeff Sheehy Jeff Sheehy is a former member of the San Francisco Board of Supervisors representing Supervisorial District 8. He was appointed to the Board in January 2017 by then-mayor Ed Lee to succeed Supervisor Scott Wiener...
Doc 2(Title: "Jeff Sheehy") ... Following Scott Wiener's departure from the San Francisco Board of Supervisors due to his election to the California State Senate in 2016, Sheehy was appointed to fill out the remainder of his term by San Francisco Mayor Ed Lee...
Doc 3(Title: "Ed Lee (politician)") ... At the January 7 meeting, the old board voted 10–1 to elect Lee as mayor, with outgoing Supervisor Chris Daly casting the lone ""no"" vote...\textcolor{orange}{</retrieval>}

\textcolor{magenta}{<information>} Jeff Sheehy was appointed to the San Francisco Board of Supervisors in January 2017 by then-mayor Ed Lee. Ed Lee was elected as mayor by the Board of Supervisors on January 7, 2011, after a vote of 10–1. There is no direct information about Ed Lee's appointment date to the Board of Supervisors, but he was elected mayor in early 2011. Therefore, Ed Lee's involvement with the Board of Supervisors predates Jeff Sheehy's appointment in 2017. \textcolor{magenta}{</information>}

\textcolor{blue}{<think>}I found out that Jeff Sheehy was appointed to the San Francisco Board of Supervisors in January  e11 by then-mayor Ed Lee. Now I need to determine which one was appointed first, Jeff Sheehy or Ed Lee.\textcolor{blue}{</think>}

\textcolor{cyan}{<search>} when was Ed Lee appointed to the board of supervisors \textcolor{cyan}{</search>}

\textcolor{orange}{<retrieval>}...\textcolor{orange}{</retrieval>}

\textcolor{magenta}{<information>} Jeff Sheehy was appointed to the San Francisco Board of Supervisors in January 2017 by then-mayor Ed Lee. Ed Lee was appointed by the Board of Supervisors on January 11, 2011, to serve out the remaining term of former Mayor Gavin Newsom after Newsom resigned. Ed Lee was elected mayor by the Board of Supervisors on January 7, 2011. Therefore, Ed Lee was appointed to the Board of Supervisors first, in 2011, well before Jeff Sheehy's appointment in 2017. \textcolor{magenta}{</information>}

\textcolor{blue}{<think>}I found out that Ed Lee was appointed to the Board of Supervisors first, in 2011, before Jeff Sheehy's appointment in 2017.\textcolor{blue}{</think>}

\textcolor{purple}{<answer>} Ed Lee \textcolor{purple}{</answer>}

\textbf{\textcolor{teal}{Correct Answer:}} Ed Lee
\end{tcolorbox}

\subsection{Sample Output From Search-R1 With De-Duplication Component}
\begin{tcolorbox}[colback=gray!5!white, breakable, enhanced]
\textbf{Question:} Who was appointed to the board of supervisors first, Jeff Sheehy or Ed Lee?

\textcolor{blue}{<think>}I need to determine if Jeff Sheehy or Ed Lee was appointed to the board of supervisors first. I'll search for it.\textcolor{blue}{</think>}

\textcolor{cyan}{<search>} who was appointed to the board of supervisors first, Jeff Sheehy or Ed Lee \textcolor{cyan}{</search>}

\textcolor{orange}{<information>}Doc 1(Title: "Jeff Sheehy") Jeff Sheehy Jeff Sheehy is a former member of the San Francisco Board of Supervisors representing Supervisorial District 8. He was appointed to the Board in January 2017 by then-mayor Ed Lee to succeed Supervisor Scott Wiener...
Doc 2(Title: "Jeff Sheehy") ...Following Scott Wiener's departure from the San Francisco Board of Supervisors due to his election to the California State Senate in 2016, Sheehy was appointed to fill out the remainder of his term by San Francisco Mayor Ed Lee...
Doc 3(Title: "Ed Lee (politician)") take their place.) ...At the January 7 meeting, the old board voted 10–1 to elect Lee as mayor, with outgoing Supervisor Chris Daly casting the lone ""no"" vote... \textcolor{orange}{</information>}

\textcolor{blue}{<think>}I found out that Jeff Sheehy was appointed to the San Francisco Board of Supervisors in January 2017 by then-mayor Ed Lee. Now I need to determine if Ed Lee was appointed to the board of supervisors first or not.\textcolor{blue}{</think>}

\textcolor{cyan}{<search>} when was Ed Lee appointed to the board of supervisors \textcolor{cyan}{</search>}

\textcolor{orange}{<information>}Doc 1(Title: "Ed Lee (politician)") ...He took office as San Francisco city administrator in 2005 and was appointed on January 11, 2011 by the Board of Supervisors to serve out the remaining term of former Mayor Gavin Newsom...
Doc 2(Title: "Ed Lee (politician)")if appointed, a statement that helped to gain support for his appointment...
Doc 3(Title: "Ed Lee (politician)")In 1991, he was hired as Executive Director of the San Francisco Human Rights Commission...
\textcolor{orange}{</information>}

\textcolor{blue}{<think>}I found out that Ed Lee was appointed to the board of supervisors in January 11, 2011. Now I can compare the appointments of Jeff Sheehy and Ed Lee to the board of supervisors.\textcolor{blue}{</think>}

\textcolor{cyan}{<search>} compare the appointments of Jeff Sheehy and Ed Lee to the board of supervisors \textcolor{cyan}{</search>}

\textcolor{orange}{<information>}Doc 1(Title: "2018 San Francisco Board of Supervisors election") ...Incumbent Supervisor Jeff Sheehy was eligible to run for reelction in the June 5, 2018 special election...
Doc 2(Title: "Ed Lee (politician)") In 2010 a vacancy in the office of mayor was impending when incumbent Gavin Newsom...
Doc 3(Title: "Kern County Board of Supervisors") 1927–34 16. George W. Parish, 1935–38 17. C.W. Harty, 1939–50 18. John W. Holt...
\textcolor{orange}{</information>}

\textcolor{blue}{<think>}I found out that Ed Lee was appointed to the board of supervisors in January 11, 2011. Jeff Sheehy was appointed to the San Francisco Board of Supervisors in January 2017 by then-mayor Ed Lee. Now I can provide the answer.\textcolor{blue}{</think>}

\textcolor{purple}{<answer>} Ed Lee \textcolor{purple}{</answer>}

\textbf{\textcolor{teal}{Correct Answer:}} Ed Lee
\end{tcolorbox}

\subsection{Prompts}

\subsubsection{Prompt to create a memory cache}

\begin{tcolorbox}[colback=gray!5!white, colframe=gray!80!black, title=GPT Information Extractor Prompt, coltitle=white, colbacktitle=gray!70!black, fonttitle=\bfseries]

    Answer the given question. \\
    You must conduct reasoning inside <think> and </think> first every time you get new information. \\
    After reasoning, if you find you lack some knowledge, you can call a search engine by <search> query </search> and it will return the top searched results between <information> and </information>. \\
    You can search as many times as your want only if you don't know the answer yet. \\
    If you find no further external knowledge needed, you can directly provide the answer inside <answer> and </answer>, without detailed illustrations. For example, <answer> xxx </answer>. Question: \{question\}

    \textbf{Task Instruction:} Your objective is to only extract relevant and helpful information needed in the reasoning process to answer the Question from the Retrieved Information. Identify factual information that is relevant to the Question and can aid in the reasoning process for the question. \\

    \end{tcolorbox}

\begin{tcolorbox}[colback=gray!5!white, colframe=gray!80!black, title=GPT Prompt, coltitle=white, colbacktitle=gray!70!black, fonttitle=\bfseries]
    Guidelines: \\
    \textbf{1. Extract Relevant Information: }\\
    - Select only the relevant information from the <retrieval> and </retrieval> that directly contributes to answering the question. \\

    - Ensure that the extracted information is accurate and relevant.\\
    - Add this new relevant information to the Previous Information inside <information> and </information>. \\
    - You must not remove any information, only new information can be added. \\
    \textbf{2. Output Format: }\\
    - If there is helpful information to answer the Question: Present the information beginning with <information> and ending with </information> as shown below. \\
    <information> Helpful information </information> \\

    - If there is no new helpful information to answer the Question: If there is Previous Information output the previous information otherwise output the following text. <information> No helpful information found </information>. \\
    \textbf{Inputs:} \\
    - Question: \{question\} \\
    - Retrieved Information: \{information\} \\
    - Previous Information: \{prev\_cache\} \\
    
    Now you should analyze all documents in the information and find helpful information based on the Question “\{question\}”. \\

\end{tcolorbox}

\subsubsection{Prompt for LLM Match}

\begin{tcolorbox}[colback=gray!5!white, colframe=gray!80!black, title=LLM Match Prompt, coltitle=white, colbacktitle=gray!70!black, fonttitle=\bfseries]

    You are an expert evaluator to judge if the model's predicted answer correctly matches any of the ground truth answer. Carefully consider the meaning and correctness. Minor variations in wording are acceptable if the predicted answer conveys the same information as the ground truth. \\
    
    Given:\\
    The predicted answer. \\
    The ground truth answer. \\
    
    Task: \\
    Score 0 or 1 based on the semantic similarity of predicted and ground truth answer. \\
    
    Notes:\\
    Evaluate only semantic similarity, not factual correctness. \\
    
    Scoring: \\
    0 - The predicted answer is not equivalent to ground truth, incomplete in a meaningful way, or diverges in meaning from the ground truth. \\
    1 - The predicted answer is semantically similar or conveys the same meaning as ground truth \\
    
    Output: \\
    Score: X \\
    Justification: [Concise 1-2 sentence justification] \\
    
    Input: \\
    Predicted Answer: \{the predicted answer\} \\
    Ground Truth Answers: \{a collection of correct answers\} \\
    
\end{tcolorbox}

\subsubsection{Prompt for to Score how well the model has reasoned on the retrieved information}

\begin{tcolorbox}[colback=gray!5!white, colframe=gray!80!black, title=System Prompt, coltitle=white, colbacktitle=gray!70!black, fonttitle=\bfseries]
    You are an expert evaluator rating how well a model's reasoning extracts and uses relevant information from given search results to answer the original question. \\
    
    Given: \\
    The original question \\
    The retrieved search information \\
    The model's reasoning after retrieval \\
    
    Task: \\
    Score 1-5 how well the reasoning reflects extraction and use of the most relevant info to answer the question. \\
    
    Notes: \\
    Evaluate only relevance and usage of retrieved info, not factual correctness. \\
    Reasoning may include prior retrieval info if clearly relevant. \\
    Ignore irrelevant details, even if from the retrieved data. \\
    
    Scoring: \\
    5 - Uses all key relevant info accurately. \\
    4 - Uses most relevant info; minor omissions. \\
    3 - Uses some relevant info; misses significant details or has minor irrelevant parts. \\
    2 - Uses little relevant info; many important details missing. \\
    1 - Fails to use relevant info or includes mostly irrelevant/misleading content. \\
    
    Output: \\
    Score: X \\
    Justification: [Concise 1-2 sentence justification]
\end{tcolorbox}

\begin{tcolorbox}[colback=gray!5!white, colframe=gray!80!black, title=User prompt template, coltitle=white, colbacktitle=gray!70!black, fonttitle=\bfseries]
    Evalute the following input to provide a score and justification:\\
    Question: \{question\} \\
    Information: \{information\} \\
    Reasoning: \{think\} \\
\end{tcolorbox}

\subsubsection{Heatmap with the number newly retrieved documents at each search iteration for the Search-R1 baseline. }
\begin{figure}[!htb]
    \centering
    \includegraphics[width=1\linewidth]{figures/heatmap.png}
    \label{fig:heatmap}
\end{figure}

\subsubsection{Heatmap with the number newly retrieved documents at each search iteration for the Information Extractor.}
\begin{figure}[!htb]
    \centering
    \includegraphics[width=1\linewidth]{figures/download-2.png}
    \label{fig:heatmap}
\end{figure}

% \subsubsection{Prompt for Determining Document Helpfulness}

% \begin{tcolorbox}[colback=gray!5!white]
%     You are a document snippet relevance judge. Given a question inside <question></question>, and a text chunk inside <document></document> retrieved from a dense retriever, evaluate how useful the document is in helping answer the query. Assign a score from 0 to 4 using the following criteria: \\
%     0 – Not Relevant: No connection to the query. \\
%     1 – Slightly Relevant: Minimal overlap; mostly unhelpful.\\
%     2 – Somewhat Relevant: Weak signal but on-topic. \\
%     3 – Relevant: Clearly contributes useful content. \\
%     4 – Highly Relevant: Strong, directly useful information. \\
    
%     Output your answer as a json with the format \{"score": < 0 | 1 | 2 | 3 >, "explanation": "<brief justification>"\}
% \end{tcolorbox}

% \subsubsection{Prompt for Determining if Query is Multi-goal}

% \begin{tcolorbox}[colback=gray!5!white]
%     You are an assistant that determines if a search query (inside <search> and </search>) is multi-goal.
%     Choose "yes" if the query contains more than one subject, entity, aspect, or sub-question, even if related.
%     Choose "no" if it's narrowly focused on a single subject with no additional elements or comparisons.
%     Be strict: if in doubt or if multiple ideas/entities are present, default to "yes".
    
%     Output as JSON: \{"judgement": < yes | no >, "explanation": "<brief justification>" \}

% \end{tcolorbox}
